# Supplementary material for: Efficient Learning and Decoding of the Continuous-Time Hidden Markov Model for Disease Progression Modeling
Source: arXiv:2110.13998 source file (2021-10-26)
Supplement: Supplementary file 1 [file CTHMM_decode_appendix.tex]

\section{Search for maximum likelihood state and duration sequences}

\label{sec:decode_max_like}

In \cite{Perkins2009NIPS}, a trajectory of the CTMC is a sequence of states along with the dwell time in all but the last state: $U = (s_0, \tau_0, s_1, \tau_1, ..., s_{k-1}, \tau_{k-1}, s_k)$. This represents that the system enters state $s_0$ at the beginning and where it stays for $\tau_0$ time, then goes to $s_1$, and stays for $\tau_1$ and so on. 
	Eventually, the system hits state $s_k$ and remains there. Let $U_t = (s_0, \tau_0, s_1, \tau_1, ..., s_{k_t-1}, \tau_{k_t-1}, s_{k_t})$ be a random variable describing the trajectory of the system up until time $t$.
	This represents that there are $k_t$ state transitions up until time $t$, where $k_t$ itself is also a random variable.
	
	Given the initial state $s$, a total time $t$, the likelihood of a particular trajectory $U$ is shown as\ cite{}:
	\[L(U_t = U | s_0=s) = 
	\begin{cases} 0 & \mbox{if } s_0 \neq s \mbox{ or } \sum_{i=0}^{k-1} t_i > t \\ 
(\prod_{i=0}^{k-1} q_{s_i} e^{-q_{s_i} t_i} v_{s_i, s_{i+1}} ) (e^{-q_{s_k} (t - \sum_i \tau_i}) & \mbox{otherwise } \end{cases}  \]
The condition $\sum_{i=0}^{k-1} t_i > t$ in the first line means that the likelihood is zero if the chain has total time larger than $t$. Otherwise, in the second case
the first parenthesis $(\prod_{i=0}^{k-1} q_{s_i} e^{-q_{s_i} t_i} v_{s_i, s_{i+1}} )$ represents the likelihood of the dwell time until state $s_{k-1}$ and the state transitions in the sequence. The second parentheses $(e^{-q_{s_k} (t - \sum_i \tau_i})$ accounts for the probability that the dwell time in the last state does not finish before time $t$.

The end-conditioned most likely trajectory problem can be formulated as:
\[ arg~ max_U ~~ L(U_t = U | s(0)=s, s(t) = s^{'})  \]
where $s$ and $ s^{'}$ are the two given end-states, and $t$ is the given total time.\\

\begin{itemize}
\item \textbf{Find the most likelihood dwell time for a given state sequence:} 
	In this setting, the optimization problem becomes:
	\[ arg~ max_{(\tau_0, ..., \tau_{t_{k-1}})} ~~ L(U_t = U | s_0, s_1, ...., s_k)  \mbox{~~~~s.t.~~} \sum_i^{k-1} {t_i}< t \]
    
    In  \cite{Perkins2009NIPS}, it is shown that when given a particular state sequence, if state $s_i$ has the largest expected dwell time (i.e., has the smallest holding time parameter $q_i$), then the most likely setting of dwell time is derived by putting all of the time $T$ in state $s_i$ (the slowest state), and all other transitions happen instantaneously.
    This result is not unintuitive, but is dissatisfying in the sense that the resulting most likely set of dwell time is not typical, since none are close to their expected value.
    
\item    \textbf{Find the most likely state sequence for give end-states and total time:}	        
    With the solution for the above problem that all the times goes into the slowest state, one can now finds the most likely state sequence that maximize the likelihood using the derived formula:    
\[ arg~ max_{(\tau_0, ..., \tau_{k-1})} ~~ L(U_t = U | s_0 = s(0))  =  (\prod_{i=0}^{k-1} q_{s_i} e^{-q_{s_i} t_i} v_{s_i, s_{i+1}} ) e^{(min_{i=0}^k q_{s_i})t}. 
\]
    The solution can be found using dynamic programming. In order to build the maximum likelihood paths of increasing length, one finds the best ways of extending the shorter paths  \cite{Perkins2009NIPS}.
    The main difference here to other typical dynamic program problems is to remember not just the current score, the current end-state, but also the smallest holding time parameter $q$ along the path.
    The running time of this algorithm is $O(K|S|^3)$, where $K$ is the number of state jumps, which can be limited to be a preset value.
    
\item 	\textbf{Situations where maximum likelihood trajectory is not well-defined:}    
    It is analyzed in  \cite{Perkins2009NIPS} that if a CTMC has a cycle of states $(s_0, s1, ..., s_k = s_0)$ such that 
\[ \prod_{i=0}^{k-1} v_{s_i, s_{i+1}} q_{s_i} \geq 1 \],
     than maximum likelihood trajectories do not exist.
    A sequence of trajectories with ever-increasing likelihood can be found if the cycle is reachable. 
    Thus, before seeking the maximum likelihood trajectories from a starting state $s$, 
    one should check if the graph has a cycle having the stated property.
    This can be done by setting the weight as $log v_{s_1, s_2} q_{s_1}$ for the edge $s_1$ to $s_2$, and check whether the graph contains a positive-weight cycle, which needs polynomial time computations.
\end{itemize}
considering all duration assignments

\section{Related Statistics: computation of total-time-conditioned state sequence probability}

\label{sec:effi_statepath_prob}

Here, the goal is to compute the probability of a state sequence $G = (s_1, ..., s_n)$ given the total spanning time $t$. This can be formulated as:
\begin{align}
p( G = (s_1, ..., s_n) | t) = & (\prod_{i=1}^{n-1} v_{s_i, s_{i+1}} )  p( \sum_{i=1}^{n-1} \tau_i < t \leq \sum_{i=1}^n \tau_i | G = (s_1, ..., s_n))  
\end{align}
where $n$ is the length of $G$, $v_{s_i, s_{i+1}}$ is the state transition probability, and $\tau_i$ is the duration in each state $s_i$. 

Note that $p( \sum_{i=1}^{n-1} \tau_i \leq t \leq \sum_{i=1}^n \tau_i | G)$ can be evaluated using matrix exponential on an auxiliary $\hat{Q}$ matrix constructed using only the states along the state path (Eqn. (4)(5) in \cite{Hajiaghayi2014}). In detail, if $G = (s_1, \cdots, s_n)$, we construct an auxiliary $(n+1) \times (n+1)$ rate matrix $\hat{Q}$ as follows:
\begin{align}
\hat{Q} = \begin{bmatrix}
-q_{s_1} & q_{s_1}  & 0            & \cdots &  0  & 0  \\
0             & -q_{s_2} & q_{s_2} & \cdots &  0  & 0  \\    
\cdots & \cdots & \cdots & \cdots & \cdots & \cdots \\
0 & 0 & 0 & \cdots & -q_(s_n) & q_{s_n} \\
0 & 0 & 0 & \cdots & 0 & 0 \\
\end{bmatrix}_{(n+1)\times(n+1)}
\end{align}
where $q_{s_k} = \sum_{i, i \neq k} q_{s_k, s_i}$ is the holding time parameter of state $s_k$. This matrix has the structure that only the transition from $s_i$ to $s_{i+1}$ is set positive at the $(i,i+1)$ entry in $\hat{Q}$. It has be shown in \cite{Hajiaghayi2014} that
\begin{align}
p( \sum_{i=1}^{n-1} \tau_i \leq t \leq \sum_{i=1}^n \tau_i | G) =  (e^{\hat{Q}  t})_{1, n}
\end{align}
which is a matrix exponential operation on the auxiliary matrix $\hat{Q}$.

\textbf{Closed-form formulation for the $(1,n)$ entry of $e^{\hat{Q} t}$:}
We find that the $(1,n)$th entry of $e^{\hat{Q} t}$ has closed-form via \textit{Laplace transformation}\footnote{This is a collaborative work with Shuang Li and Le Song, who derive this exact closed-form.}. The results are as below (For notation simplicity, we write $q_{s_i}$ as $q_i$):

\begin{itemize}
	\item If $q_i, i = 1,...,n$ are distinct, we have
	\begin{align*}
	(e^{\hat{Q} t})_{1,n} =  \frac{1}{q_n}   \sum_{i=1}^n [ ( \prod_{j=1,j \neq i}^n \frac{q_j}{q_j - q_i} ) q_i e^{-q_i  t} ]
	\end{align*}				
	\item If $q_i, i = 1,...,n$ are not distinct, without loss of generality, we assume $q_1 = q_2 = ... = q_p$, and $q_{p+1} \neq q_{p+2} ... \neq q_n$, then we have the form below:
	\begin{align*}
	(e^{\hat{Q}  t})_{1,n} =  ( \frac{a_{11}}{(p-1)!} t^{p-1} + \frac{a_{12}}{(p-2)!} t^{p-2} + ... + a_{1p}) e^{-q_1 t} + A_{p+1} e^{-q_{p+1}t} + ... + A_n e^{-q_n t}		
	\end{align*}
\end{itemize}
Below we list some steps to derive $(e^{\hat{Q}  t})_{1,n}$ when $q_i$ are distinct using \textit{Laplace Transform} and the \textit{Inverse Laplace Transform} by \textit{Partial Fraction Expansion} as below:
\begin{align*}
(e^{\hat{Q}  t})_{1,n} = \mathbb{F}^{-1} ( \mathbb{F}( (e^{\hat{Q}  t})_{1,n} ) )
\end{align*}
where $\mathbb{F}^{-1}$ is \textit{Laplace Transform} and $\mathbb{F}^{-1}$ is \textit{Inverse Laplace Transform}.
\begin{align*}
\mathbb{F}(s) = \mathbb{F} (e^{\hat{Q}  t})_{1,n} = (sI - \hat{Q})^{-1}_{1,n} = \frac{q_1 q_2 ... q_{n-1}}{(s+q_1)(s+q_2)...(s+q_n)}
\end{align*}

If all  $q_i, i = 1,...,n$ are distinct, then we have
\begin{align*}
\mathbb{F}(s) = \frac{A_1}{(s+q_1)} + \frac{A_1}{(s+q_2)} + ... + \frac{A_{n-1}}{(s+q_{n-1})} + \frac{A_{n}}{(s+q_{n})} (Partial~Fraction~Expansion)
\end{align*}
, where
\begin{align*}
A_i = lim_{s \rightarrow -q_i} (s+q_i) \mathbb{F}(s) = \frac{q_1 q_2 ... q_{n-1}}{(-q_i+q_1)...(-q_i+q_{i-1})(-q_i+q_{i+1})...(-q_i+q_n) }.
\end{align*}
Then we have
\begin{align*}
(e^{\hat{Q}  t})_{1,n} &= \mathbb{F}^{-1} ( \mathbb{F}(s)) 
= A_1 e^{-q_1 t} + A_2 e^{-q_2 t} + ... + A_n e^{-q_n t} \\
& = \frac{1}{q_n}   \sum_{i=1}^n [ ( \prod_{j=1,j \neq i}^n \frac{q_j}{q_j - q_i} ) q_i e^{-q_i  t} ]
\end{align*}

\textbf{Comparison of time complexity:}

Here, we compare the time complexity of computing the state sequence probability given a total using a direct matrix exponential method and the closed-form expression we derived. The comparison is listed in Table \ref{table:time_path_prob}. The direct method means that to compute $(e^{\hat{Q}  t})_{1,n}$ by computing the matrix exponential and then read the $(1,n)$ entry, which needs $O(n^3)$ time. Clearly, our closed-form results only $O(n^2)$ time, but it need that all $q_i$ are distinct.

\begin{table*}[!htb]
	\centering	
	
	\caption{
		Time complexity comparison of all methods in evaluating time-conditioned path probability ($n$: number of states in the path)
	}	
	\begin{tabular}{|l||l||l|}
		\hline
		Complexity & direct-expm & Ours \\ \hline \hline
		Time & $O(n^3)$ & $O(n^2)$ \\ \hline \hline
		Prerequisite & none & $q_i$ distinct \\ \hline		
	\end{tabular}	 
	\label{table:time_path_prob}
\end{table*}

\section{A closed-form in computing path-and-total-time conditioned expected state duration}

\label{sec:effi_state_expect}

To the best of our knowledge, we have not found any literature that explicitly write down the closed-form and methods for computing expected state duration for a \textit{path-conditioned} CTMC. We derive a closed-form formulation for computing these path-conditioned statistics, which is applicable when $q_i$ for the states in the path are distinct. We also compare the time complexity of using our closed-form to using the three alternative methods (Expm, Unif, Eigen) which are originally used in end-state conditioned cases, to compute path-conditioned statistics by applying on an auxiliary matrix according to the state path.

%but fo apply on the auxiliary matrix constructed according to the state path.

% Here, our derivation of the expected state duration is inspired by the paper \cite{} % phase-type

We now explain our derived closed-form in detail\footnote{This is a collaborative work with Shuang Li and Le Song.}. Given a state sequence $G = (s_1, ..., s_n)$, a total duration $t$, the computation of the expected state duration $\tau_k$, for state $k = 1,...,n$ is as below:
\begin{align}
	& E (\tau_k | G , \sum_{i=1}^{n-1} \tau_{i} \le t < \sum_{i=1}^{n} \tau_i ) 
	= E [\int_{0}^{t} \mathbf{1} (S_u = s_k) du | G, \sum_{i=1}^{n-1} \tau_{i} \le t < \sum_{i=1}^{n} \tau_i  ] \\
	&= \int_0^t p(S_u = s_k | G , \sum_{i=1}^{n-1} \tau_{i} \le t < \sum_{i=1}^{n} \tau_i ) du \\
	&= \frac{\int_0^t (e^{\tilde{Q}_{k,A} u})_{1,k}  (e^{\tilde{Q}_{k,B} (t-u)})_{1,n-k+1} du}{ (e^{\tilde{Q} t})_{1,n}} \\
	&= \frac{\int_0^t   [ a_{k,1}  e^{-q_1 u} + \cdots + a_{k,k} e^{-q_k u} ] \cdot [b_{k,k} e^{-q_k (t-u)} + \cdots + b_{k,n} e^{-q_n (t-u)}] du }{(e^{\tilde{Q} t})_{1,n}} \\
	&=  \frac{( \sum_{i=1}^k \sum_{j=k, i \neq j}^{n} a_{k,i} b_{k,j} \frac{e^{-q_i t} - e^{-q_j t}}{-q_i + q_j}  ) + t (a_{k,k} b_{k,k}  e^{-q_k t})}{\frac{1}{q_n} \sum_{i=1}^{n} \bigg[ ( \prod_{j=1, j \neq i}^n \frac{q_j}{q_j-q_i} ) q_i e^{-q_i t} \bigg] }
	\label{equ:tau}
\end{align}
where $q_i = \sum_{i \neq j} q_{ij}$ are the holding time parameters, $\tilde{Q}$ is the auxiliary matrix for the entire state path:
% Q
\begin{align}
	\tilde{Q} & = \begin{bmatrix}
		-q_1 & q_1 & 0 & \cdots & 0 & 0 \\
		0 & -q_2 & q_2 & \cdots & 0 & 0 \\
		\cdots & \cdots & \cdots & \cdots & \cdots & \cdots \\
		0 & 0 & 0 & \cdots & -q_n & q_n \\
		0 & 0 & 0 & \cdots & 0 & 0 \\
	\end{bmatrix}_{(n+1)\times(n+1)},
\end{align}
, $\tilde{Q}_{k,A}$ is the auxiliary matrix for the partial state path from the first state to the $k$th state, 
% QA
\begin{align*}
	%\footnotesize
	\tilde{Q}_{k,A} = \begin{bmatrix}
		-q_1 & q_1 & 0 & \cdots & 0 & 0 \\
		0 & -q_2 & q_2 & \cdots & 0 & 0 \\
		\cdots & \cdots & \cdots & \cdots & \cdots & \cdots \\
		0 & 0 & 0 & \cdots & q_k & q_k \\
		0 & 0 & 0 & \cdots & 0 & 0 \\
	\end{bmatrix}_{(k+1)\times(k+1)},
\end{align*}
, and $\tilde{Q}_{k,B}$ is the auxiliary matrix for the partial state path from the $(k+1)$th state to the last state (the $n$th state):
\begin{align*}
	\tilde{Q}_{k,B} = \begin{bmatrix}
		-q_k & q_k & 0 & \cdots & 0 & 0 \\
		0 & -q_{k+1} & q_{k+1} & \cdots & 0 & 0 \\
		\cdots & \cdots & \cdots & \cdots & \cdots & \cdots \\
		0 & 0 & 0 & \cdots & -q_n & q_n \\
		0 & 0 & 0 & \cdots & 0 & 0 \\
	\end{bmatrix}_{(n-k+2)\times(n-k+2)}
\end{align*}
We also have the closed-form expression for $(e^{\tilde{Q} t})_{1,n}$ derived from the previous section as follows:
\begin{align}
	& (e^{\tilde{Q} t})_{1,n} = \sum_{i=1}^{n} \bigg[ ( \prod_{j=1, j \neq i}^n \frac{q_j}{q_j-q_i} )  \frac{q_i}{q_n}  e^{-q_i T} \bigg] 
	= \sum_{i=1}^{n} c_i e^{-q_i T}
\end{align}
where  $ c_i = ( \prod_{j=1, j \neq i}^n \frac{q_j}{q_j-q_i} )  \frac{q_i}{q_n}$. Finally, the terms $a_{k,i}$ and $b_{k,j}$ are defined as:
\begin{align}
	\begin{cases}
		a_{k,i} = \frac{q_i}{q_k}  (\prod_{m=1, m \neq i}^k \frac{q_m}{q_m - q_i})  &  k = 1, \cdots, n   ;  \text{  } i = 1, \cdots, k\\
		b_{k,j} = \frac{q_j}{q_n}  (\prod_{m=k, m \neq j}^n \frac{q_m}{q_m - q_j}) & k = 1, \cdots, n ; \text{  }  j = k, \cdots, n \\ 
	\end{cases}
\end{align}
which are derived from the closed-form expression for $(e^{\tilde{Q} t})_{1,n}$.

\textbf{Efficient computation of the expected duration for each state in the state path}:
we can derive the recursive relation between $a_{k,i}$ and $a_{k-1,i}$, and also $b_{k,j}$ and $b_{k+1,j}$, so that the computation of these coefficients can be efficient:
\begin{align}
	\begin{cases}
		a_{k,i} = a_{k-1,i} \frac{q_{k-1}}{q_k - q_i}  &  k = 1, \cdots, n   ;  \text{  } i = 1, \cdots, k\\
		b_{k,j} = b_{k+1,j} \frac{q_{k}}{q_k - q_j} & k = 1, \cdots, n ; \text{  }  j = k, \cdots, n \\ 
	\end{cases}
\end{align}

\textbf{Time complexity analysis:}
The time complexity in computing all $\tau_k$, $k=1,...,n$, where $n$ is the length of the inner path is $O(n^3 / 6)$. The detailed analysis is as follows. First,
the computation of all required $a_{k,i}$ and $b_{k,j}$ from the derived recursive form needs $O(n^2)$. Second, the computation of the common denumerator requires $O(n^2)$. Third, the computation of the numerator for one $\tau_k$ using the precomputed $a_{k,i}$ and $b_{k,j}$, requires  $k(n-k) = O(n^2)$. Finally, the computation of the numerator for all $\tau_k$ needs $\sum_{k=1}^n k(n-k) = (n^3-n)/6 = O(n^3/6)$.

Thus, evaluating just one expected state duration requires $O(n^2)$ computations, and evaluating all expected state durations along the path needs $O(n^3)$ ($n$ is the path length).

\textbf{Comparison of time complexity}

We compare the time complexity of computing the expected state durations given the state path and a total time from the three alternative methods (Expm, Unif, Eigen) and our closed-form solution. The three alternative methods \textit{(Expm, Unif, Eigen)} are originally used in computing the end-state conditioned statistics (see more details in Chapter 3). To use them for computing path-conditioned statistics, we only need to construct the auxiliary matrix $Q$ using the state path as the new rate matrix, and the remaining formulations are the same for calculating the end-state and path conditioned statistics. 

The time complexity comparison is listed in Table \ref{table:compare_time_expect_duration}. Our closed-form expression have only $O(n^2)$ time in computing one expected state duration, while all other methods require at least $O(n^3)$ as these alternative methods all involve matrix multiplications. When computing the expected duration for all states along the path, our close-form method has $O(n^3)$ complexity, and is more efficient than \textit{Expm and Unif} methods. However, our method and \textit{Eigen} both have prerequisite of its use, while \textit{Expm} and \textit{Unif} are more general.

%in evaluating path-and-time conditioned state expected duration}:

\begin{table*}[!htb]
	
	{\footnotesize
		\centering	
		
		\caption{
			Time complexity comparison of all methods in evaluating path-and-time conditioned expected state durations.
			(n: number of states in the path, $M$: the truncation point for \textit{Unif}, set as $\ulcorner 4 + 6 \sqrt{\hat{q} t} + (\hat{q} t) \urcorner$, where $\hat{q} = max_i ~q_i$ for states in the path, and $t$: the total time).
		}	
		\label{table:compare_time_expect_duration}
		\begin{tabular}{|l||l|l|l||l|}
			\hline
			Complexity & Expm & Unif & Eigen & Our Closed-Form \\ \hline \hline
			For one state & $O((2n)^3)$ & $O(M n^3 + M^2)$ & $O(n^3 + n^2)$ & $O(n^2)$  \\ \hline
			For all states & $O(n(2n)^3)=O(n^4)$ & $O(M n^3 + M^2 n)$ & $O(n^3 + n^3)$ & $O(n^3)$  \\ \hline \hline
			Prerequisite & none & none & Q diagonalizable & $q_i$ distinct \\ \hline		
		\end{tabular}	
	} 
	
\end{table*}
